# Supplementary material for: Mip-NeRF RGB-D: Depth Assisted Fast Neural Radiance Fields
Source: arXiv:2205.09351 source file (2022-11-07)
Supplement: Supplementary file 1 [file content_supp.tex]

%%%%%%%%%%%%%%%%%%%%%%%%%%%%%%%%%%%%%%%%%%%%%%%%
\section{Model Parameters / Optimization Details}
